# Supplementary material for: Dead or Murdered? Predicting Responsibility Perception in Femicide News Reports
Source: arXiv:2209.12030 source file (2022-09-24)
Supplement: Supplementary file 1 [file appendix.tex]

\appendix

\section{Appendix}
\label{sec:appendix}

\subsection{Questionnaire Results}
\label{sub:app-questionnaire}

Figures~\ref{fig:app-blame-density} through~\ref{fig:app-focus-density} show the distribution of z-scored perception scores per question and attribute.

\begin{figure}[p]
    \centering
    \includegraphics[height=\textheight]{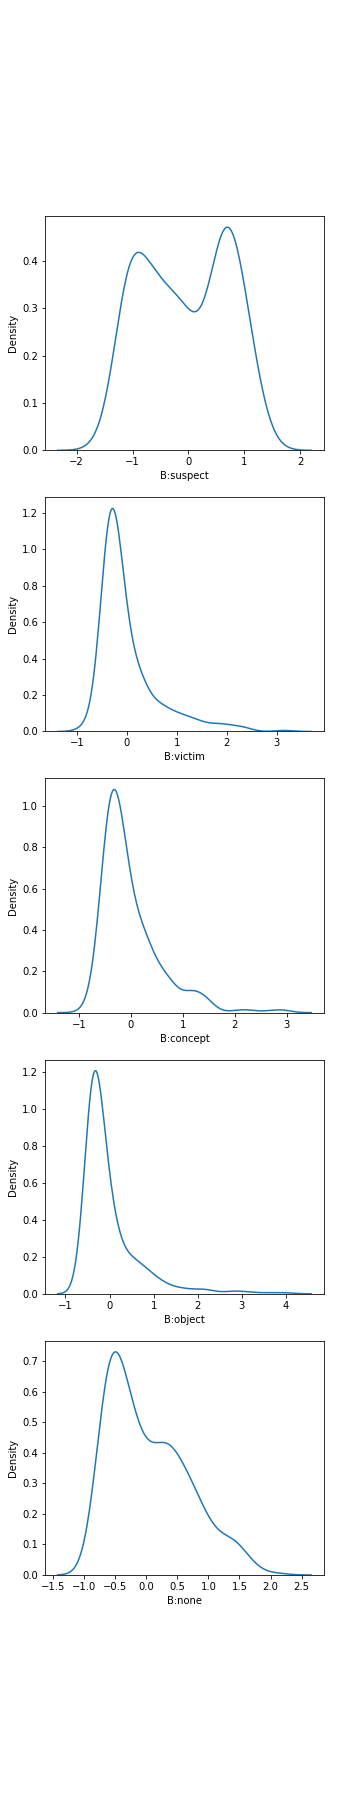}
    \caption{Density plot of aggregated z-scores for \textit{blame}}
    \label{fig:app-blame-density}
\end{figure}

\begin{figure}[p]
    \centering
    \includegraphics[height=.8\textheight]{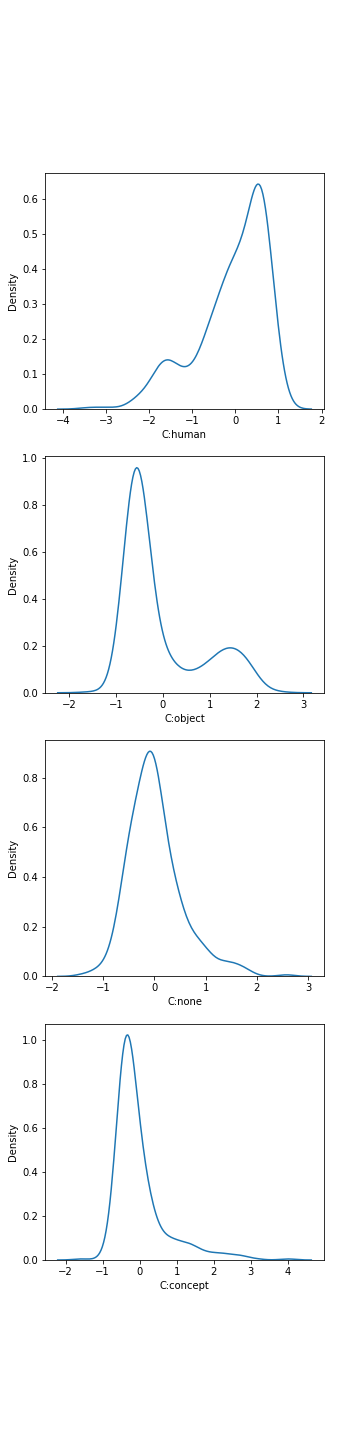}
    \caption{Density plot of aggregated z-scores for \textit{cause}}
    \label{fig:app-cause-density}
\end{figure}

\begin{figure}[p]
    \centering
    \includegraphics[height=.8\textheight]{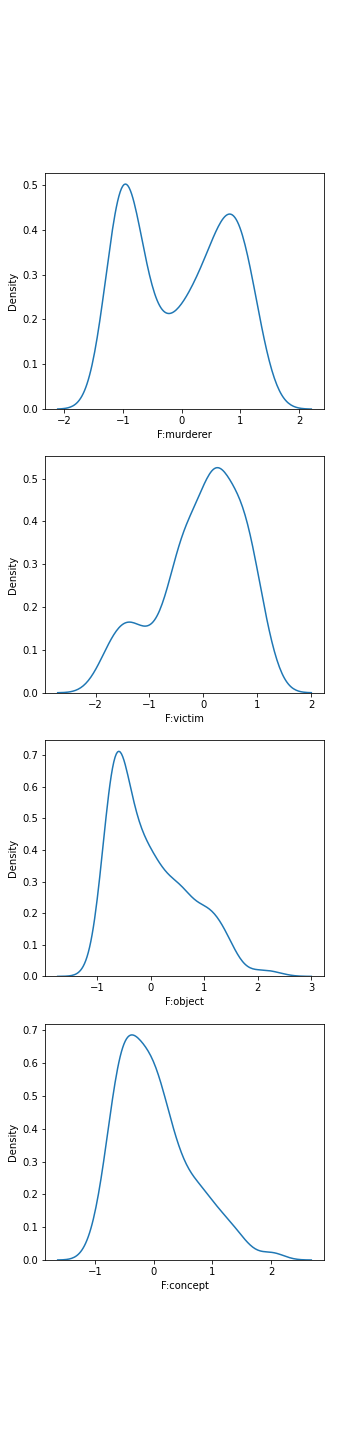}
    \caption{Density plot of aggregated z-scores for \textit{blame}}
    \label{fig:app-focus-density}
\end{figure}

\subsection{Transformer models}
\label{sec:app-hf-models}

Below are details about the exact versions of the pre-trained transformer models that we used:

\begin{itemize}
    \item \textbf{Italian BERT XXL (BERT-IT)}: published by the Bavarian State Library at \url{https://huggingface.co/dbmdz/bert-base-italian-xxl-cased}. N.B.: `XXL' refers to the corpus size, not the size of the model itself.
    \item \textbf{BERTino}: \url{https://huggingface.co/indigo-ai/BERTino}; this is a DistilBERT model, using Italian BERT XXL as its teacher but trained on a different corpus.
    \item \textbf{Multilingual BERT (mBERT)}:\\ \url{https://huggingface.co/bert-base-multilingual-cased}
    \item \textbf{Multilingual DistilBERT}:\\ \url{https://huggingface.co/distilbert-base-multilingual-cased}
    \item \textbf{XLM-RoBERTa}:\\ \url{https://huggingface.co/xlm-roberta-base}
\end{itemize}
